# Supplementary material for: A Dataset for Tracking Entities in Open Domain Procedural Text
Source: arXiv:2011.08092 source file (2020-10-31)
Supplement: Supplementary file 1 [file appendix.tex]

% \newpage
\appendix

\section*{Appendix A: Mechanical Turk Interface for acquiring \ourdata{} annotations}
We used the following crowd sourcing design through Amazon Mechanical Turk for data collection. General instructions for the task are shown in Figure \ref{fig:1} followed by an  example annotations in Figure \ref{fig:2}. For a given WikiHow article, annotators were asked to describe up to six state changes for each step. Next, we present example HITs for the procedure ``how to make Mediterranean coffee'' step 1 to 4 in Figures \ref{fig:3}, \ref{fig:4}, \ref{fig:5} and \ref{fig:6}.

% \begin{figure*}[!h]
%  \centering
%     %%% note: In the first figure, use 0 Y_low, 1140, 7530 for viewport. i.e., y_low is the only variable
%     %\includegraphics*[viewport=0 6300 1140 7530,width=1.0\textwidth]{hit_data_collection.png}
%     \includegraphics*[viewport=0 6600 1140 7530,width=1.0\textwidth]{figures/hit_data_collection.png}
% \end{figure*}

% \begin{figure*}[t]
%  \centering
%   %%% note: in the second and following figures, use 0, y-1765, 1140, y for viewport. i.e., y is the only variable.
%   % 1 page has 1765 pixel (in y)
%     \includegraphics*[viewport=0 4535 1140 6300,width=1.0\textwidth]{figures/hit_data_collection.png}
% \end{figure*}

\begin{figure*}[!h]
    {\includegraphics[width=0.95\textwidth]{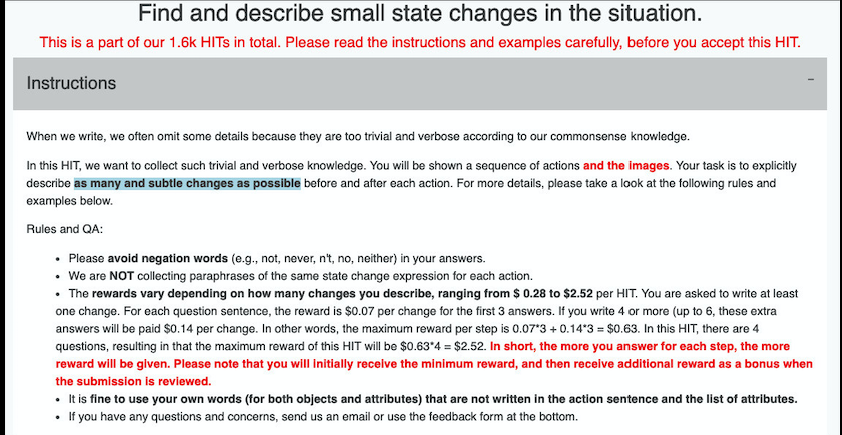}}
    \caption{Annotation task instructions.}
    \label{fig:1}
\end{figure*}

\begin{figure*}[!h]
    {\includegraphics[width=0.95\textwidth]{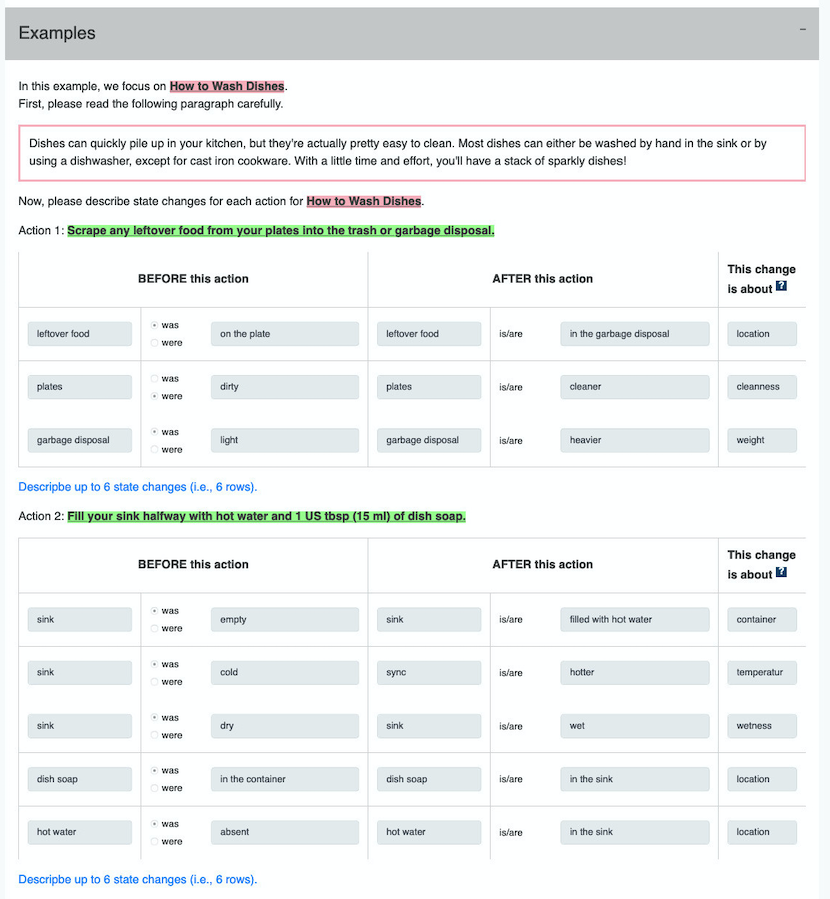}}
    \caption{Illustrative example showing ideal annotations for a procedure ``How to Wash Dishes''. }
    \label{fig:2}
\end{figure*}

\begin{figure*}[!h]
    {\includegraphics[width=0.95\textwidth]{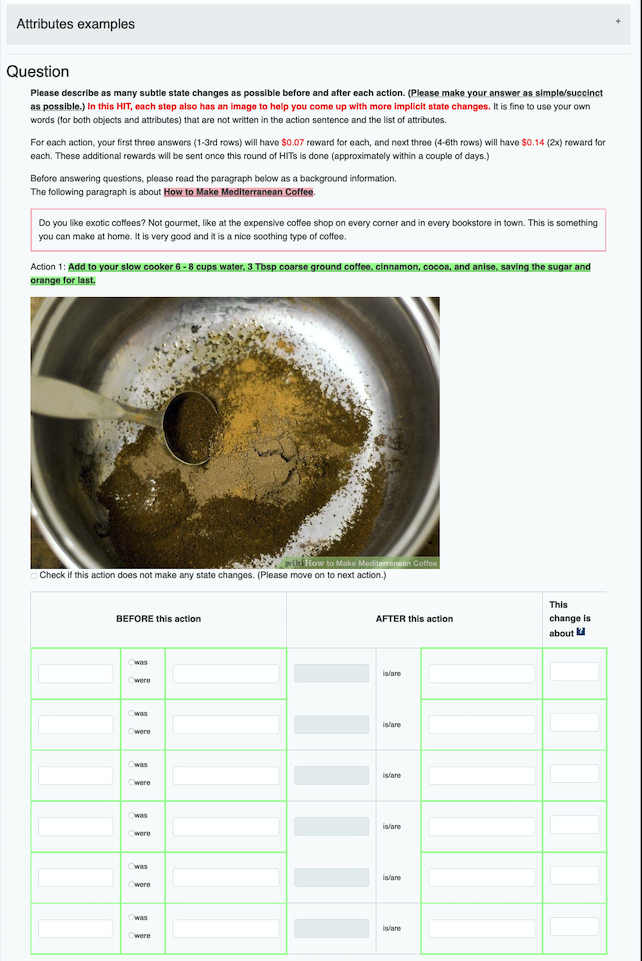}}
    \caption{Example HIT for mechanical turkers. Procedure: ``how to make Mediterranean coffee'' Action 1.}
    \label{fig:3}
\end{figure*}

\begin{figure*}[!h]
    {\includegraphics[width=0.95\textwidth]{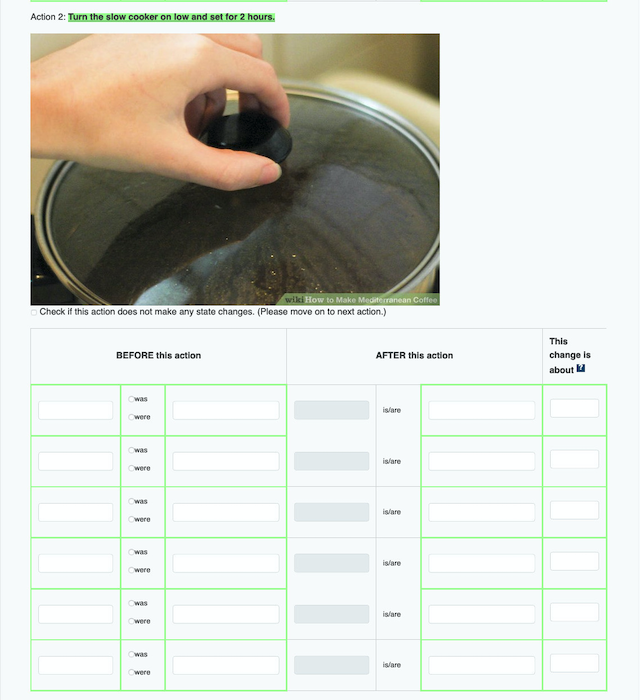}}
    \caption{Example HIT for mechanical turkers. Procedure: ``how to make Mediterranean coffee'' Action 2.}
    \label{fig:4}
\end{figure*}

\begin{figure*}[!h]
    {\includegraphics[width=0.95\textwidth]{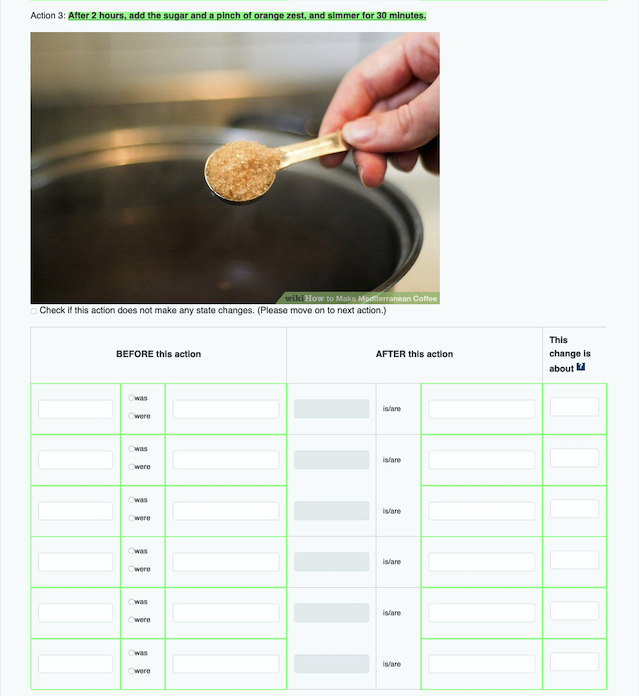}}
    \caption{Example HIT for mechanical turkers. Procedure: ``how to make Mediterranean coffee'' Action 3.}
    \label{fig:5}
\end{figure*}

\begin{figure*}[!h]
    {\includegraphics[width=0.95\textwidth]{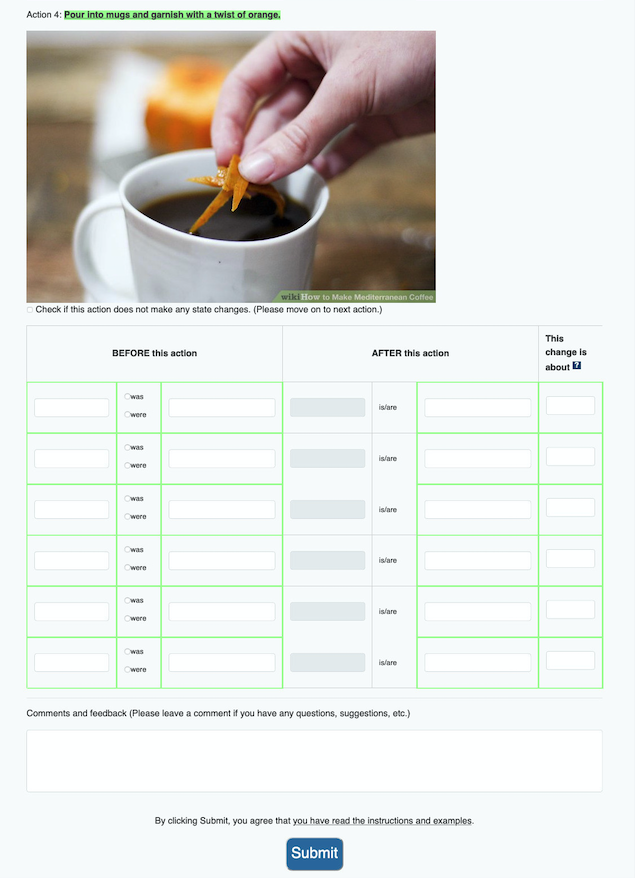}}
    \caption{Example HIT for mechanical turkers. Procedure: ``how to make Mediterranean coffee'' Action 4.}
    \label{fig:6}
\end{figure*}
